# Supplementary material for: New mixture models for decoy-free false discovery rate estimation in mass-spectrometry proteomics
Source: arXiv:2009.08023 ancillary file (2020-09-17)
Supplement: Supplementary file 1 [file sup.pdf]

# Supplementary Materials

## 1 Supporting Lemmas for the derivation of the parameter update equations

**Notation for the Lemmas**: We use $\theta$ as a placeholder for SN parameters and $\zeta$ as a placeholder for the complete model parameters; i.e., for the the top score skew normal mixture model it is the triple $(\alpha, \theta_c, \theta_1)$ and for the top two score skew normal mixture model it is the quintuple $(\alpha, \beta, \theta_c, \theta_1, \theta_2)$. "Equality after removing additive terms constant w.r.t. $a$" is denoted by $\stackrel{a}{=}$ and "equality after removing multiplicative terms constant w.r.t. $a$" is denoted by $\stackrel{a}{\propto}$. Abusing the notation, we use small letters to denote the random variable as well as its realization. $\text{HN}(0,1)$ denotes the standard normal distribution truncated below 0. $\text{N}(0,1)$ denotes the standard normal distribution. $\text{TN}(\eta, \sigma^2, \mathbb{R}_+)$ is a truncated normal distribution truncated below 0 with location and (squared) scale parameters $\eta$ and $\sigma^2$. Let

$$q(x,t,\tau,\theta) = \log\Gamma + \frac{(x-\mu)^2 - 2(x-\mu)\Delta t + (\Delta^2+\Gamma)\tau}{\Gamma}$$

And for $T_x \sim \text{TN}\big({}^{\delta}\!/\!_{\omega}(x-\mu), 1-\delta^2, \mathbb{R}_+\big)$,

$$v(x,\theta) = \mathbb{E}[T_x]$$
$$w(x,\theta) = \mathbb{E}\big[T_x^2\big]$$

$v(x,\theta)$ and $w(x,\theta)$ can be computed using Lemma 1. When $x \to -\infty$ the ratio ${}^{\phi(x)}\!/\!_{\Phi(x)}$ can be approximated as $|x|$.

**Lemma** 1. *For $T \sim \text{TN}\big(\eta, \sigma^2, \mathbb{R}_+\big)$ (truncated normal distribution, truncated below 0),*

$$E[T] = s_1(\eta,\sigma^2) = \eta + \sigma\frac{\phi(\frac{\eta}{\sigma})}{\Phi(\frac{\eta}{\sigma})},$$
$$E[T^2] = s_2(\eta,\sigma^2) = \eta^2 + \sigma^2 + \eta\sigma\frac{\phi(\frac{\eta}{\sigma})}{\Phi(\frac{\eta}{\sigma})},$$

*where $\phi$ and $\Phi$ are pdf and cdf of a standard normal distribution, respectively.*

Proof. (Johnson and Kotz, 1970)(pp. 156-158) gives the following result for truncated normal distributions. For $X \sim \text{TN}\big(\eta, \sigma^2, (a_{1},_{2}\,)\big)$,

$$E[X] = \eta - \sigma\frac{\phi(\alpha_2)-\phi(\alpha_1)}{\Phi(\alpha_2)-\Phi(\alpha_1)},$$
$$E[X^2] = \eta^2 + \sigma^2 - \sigma^2\frac{\alpha_2\phi(\alpha_2)-\alpha_1\phi(\alpha_1)}{\Phi(\alpha_2)-\Phi(\alpha_1)} - 2\eta\sigma\frac{\phi(\alpha_2)-\phi(\alpha_1)}{\Phi(\alpha_2)-\Phi(\alpha_1)},$$

where $\alpha_i = \frac{a_i-\eta}{\sigma}$

It follows that

$$E[T] = \eta - \sigma\frac{0-\phi(-\frac{\eta}{\sigma})}{1-\Phi(-\frac{\eta}{\sigma})}$$
$$= \eta + \sigma\frac{\phi(\frac{\eta}{\sigma})}{\Phi(\frac{\eta}{\sigma})}.$$

and

$$E[T^2] = \eta^2 + \sigma^2 - \sigma^2\frac{0-(-\frac{\eta}{\sigma})\phi(-\frac{\eta}{\sigma})}{1-\Phi(-\frac{\eta}{\sigma})} - 2\eta\sigma\frac{0-\phi(-\frac{\eta}{\sigma})}{1-\Phi(-\frac{\eta}{\sigma})}$$
$$= \eta^2 + \sigma^2 - \sigma\eta\frac{\phi(\frac{\eta}{\sigma})}{\Phi(\frac{\eta}{\sigma})} + 2\eta\sigma\frac{\phi(\frac{\eta}{\sigma})}{\Phi(\frac{\eta}{\sigma})}$$
$$= \eta^2 + \sigma^2 + \eta\sigma\frac{\phi(\frac{\eta}{\sigma})}{\Phi(\frac{\eta}{\sigma})}$$

**Lemma** 2. *Let $X \sim \text{SN}(\theta)$, $T \sim \text{HN}(0,1)$ and $U \sim \text{N}(0,1)$ be related by the probabilistic representation of a* SN *random variable as $X \stackrel{d}{=} \mu + \Delta T + \Gamma^{1/2}U$. Then for the joint density function $p(x,t;\theta)$,*

$$\mathbb{E}\big[\log p(X,T;\theta)|X=x;\bar\theta\big] \stackrel{\theta}{=} -\frac{1}{2}q\big(x, v(x,\bar\theta), w(x,\bar\theta), \theta\big),$$

*where the expectation is taken w.r.t. the distribution of $T$ given $X=x$ with $\bar\theta$ used as the parameter for the conditional distribution.*

Proof.

**Distribution of $T$ given $X = x$**: From the probabilistic representation of $X$, the distribution of $X$ given $T = t$ is a univariate Normal, $\mathrm{N}(\mu + \Delta t, \Gamma)$. Now, the joint distribution of $X$ and $T$ is given by

$$\begin{aligned} p(x,t) &= p(x|t)p(t) \\ &= \frac{1}{\sqrt{2\pi\Gamma}} \exp\left(\frac{-((x-\mu)-\Delta t)^2}{2\Gamma}\right) \cdot \sqrt{\frac{2}{\pi}} \exp\left(-\frac{t^2}{2}\right) I(t>0) \\ &= \frac{1}{\pi\sqrt{\Gamma}} \exp\left(\frac{-\big((x-\mu)^2 - 2(x-\mu)\Delta t + (\Delta^2+\Gamma_1)t^2\big)}{2\Gamma}\right) I(t>0) \end{aligned} \tag{1}$$

Let $\eta(x,\theta) = {}^{\delta}/_{\omega}(x-\mu)$. The conditional distribution of $T$ given $X = x$ can be derived as

$$\begin{aligned} p(t|x) &\overset{t}{\propto} p(x,t) \\ &\overset{t}{\propto} \exp\left(\frac{-\big((\Delta^2+\Gamma)t^2 - 2(x-\mu)\Delta t\big)}{2\Gamma}\right) I(t>0) \quad \text{(from Equation 1)} \qquad (2) \\ &\overset{t}{\propto} \exp\left(\frac{-\big(t^2 - 2t\eta(x,\theta)\big)}{2(1-\delta^2)}\right) I(t>0) \qquad \left(\text{because } \tfrac{\Gamma}{\Gamma+\Delta^2} = 1-\delta^2 \text{ and } \tfrac{\Delta}{\Gamma+\Delta^2} = \tfrac{\delta}{\omega}\right) \\ &\overset{t}{\propto} \exp\left(\frac{-\Big(t^2 - 2t\eta(x,\theta) + (\eta(x,\theta))^2\Big)}{2(1-\delta^2)}\right) I(t>0) \\ &\overset{t}{\propto} \exp\left(\frac{-(t-\eta(x,\theta))^2}{2(1-\delta^2)}\right) I(t>0). \end{aligned}$$

Thus $t|x \sim \mathrm{TN}\big(\eta(x,\theta), 1-\delta^2, \mathbb{R}_+\big)$

**Expectation of the log of the joint distribution**: From Equation 1 the expression for $p(x,t)$ can be written as

$$p(x,t) = \frac{1}{\pi} \exp\left(-\frac{q(x,t,t^2,\theta)}{2}\right) I(t>0).$$

Taking log and removing terms constant in $\theta$,

$$\log p(x,t) \overset{\theta}{=} -\frac{q\big(x,t,t^2,\theta\big)}{2}$$

Treating $\log p(x,t)$ as a function of random variables $X$ and $T$ and taking its conditional expectation given $X = x$ and $\bar{\theta}$,

$$\mathbb{E}\big[\log p(X,T;\theta)|X=x;\bar{\theta}\big] \overset{\theta}{=} -\frac{1}{2} q\big(x, v(x,\bar{\theta}), w(x,\bar{\theta}), \theta\big),$$

since $v(x,\theta) = \mathbb{E}[T|X=x]$ and $w(x,\theta) = \mathbb{E}\big[T^2|X=x\big]$ by definition.

**Lemma** 3. *Let $X_0$ and $X_1$ be two continuous random variables. Let $X$ be a mixture random variable defined as $X = ZX_1 + (1-Z)X_0$, where $Z \sim \mathrm{Bernoulli}(\alpha)$ for $\alpha \in [0,1]$. Then For any random variable $T$, not necessarily independent of $X$ and for any real function $h$, the following statements are true*

$$\mathbb{E}[Zh(T)|X] = p(Z=1|X) \cdot \mathbb{E}[h(T)|X, Z=1]$$
$$\mathbb{E}[(1-Z)h(T)|X] = p(Z=0|X) \cdot \mathbb{E}[h(T)|X, Z=0]$$

Proof.

By the law of iterated expectation,

$$\begin{aligned} \mathbb{E}[Zh(T)|X] &= \mathbb{E}[\mathbb{E}[Zh(T)|X,Z]|X] \\ &= \mathbb{E}[Z\mathbb{E}[h(T)|X,Z]|X] \\ &= p(Z=1|X) \cdot 1 \cdot \mathbb{E}[h(T)|X,Z=1] + p(Z=0|X) \cdot 0 \cdot \mathbb{E}[h(T)|X,Z=0] \\ &= p(Z=1|X)\mathbb{E}[h(T)|X,Z=1] \end{aligned}$$

To prove the expression for $\mathbb{E}[(1-Z)h(T)|X]$, use the same argument with $1-Z$, instead of $Z$.

**Lemma** 4. *Let $S_1$ be the random variable corresponding to the top score under the* 1SMix *model; i.e.,* $S_1 = ZX_c + (1 - Z)X_1$, *where* $X_c \sim \text{SN}(\theta_c), X_1 \sim \text{SN}(\theta_1)$ *and* $Z \sim \text{Bernoulli}(\alpha)$. *Let* $T_c, T_1 \sim \text{HN}(0,1)$ *and* $U_c, U_1 \sim \text{N}(0,1)$ *be related to* $X_c$ *and* $X_1$ *respectively by the probabilistic representation of* SN *random variable as* $X_c \stackrel{d}{=} \mu_c + \Delta_c T_c + \Gamma_c^{1/2} U_c$ *and* $X_1 \stackrel{d}{=} \mu_1 + \Delta_1 T_1 + \Gamma_1^{1/2} U_1$. *Further, let* $T = ZT_c + (1-Z)T_1$. *Then for the joint density of* $S_1, T, Z$ *given by* $p(s_1, t, z; \zeta)$,

$$
\begin{aligned}
&\mathbb{E}\big[\log p(S_1, T, Z; \zeta) | S_1 = s_1; \bar{\zeta}\big] \\
&\stackrel{\zeta}{=} \bar{p}_c(s_1)\bigg(\log\alpha - \frac{1}{2} q\big(s_1, v(s_1, \bar{\theta}_c), w(s_1, \bar{\theta}_c), \theta_c\big)\bigg) \\
&\quad + \bar{p}_1(s_1)\bigg(\log(1-\alpha) - \frac{1}{2} q\big(s_1, v(s_1, \bar{\theta}_1), w(s_1, \bar{\theta}_1), \theta_1\big)\bigg)
\end{aligned}
$$

*where $\zeta$ serves as placeholder for $(\alpha, \theta_c, \theta_1)$; the expectation is taken w.r.t. the distribution of $Z, T$ given $S_1 = s_1$ with $\bar{\zeta}$ used as the parameter for the conditional distribution;*

$$
\begin{aligned}
\bar{p}_c(s_1) &= p\big(Z = 1 | S_1 = s_1, \bar{\zeta}\big) \\
\bar{p}_1(s_1) &= p\big(Z = 0 | S_1 = s_1, \bar{\zeta}\big).
\end{aligned}
$$

Proof. The joint distribution of $S_1, T, Z$ can be written as

$$
\begin{aligned}
p(s_1, t, z) &= p(s_1, t, Z = 1)^z p(s_1, t, Z = 0)^{1-z} \\
&= [p(s_1, t | Z = 1) p(Z = 1)]^z [p(s_1, t | Z = 0) p(Z = 0)]^{1-z} \\
&= [p(X_c = s_1, T_c = t)\alpha]^z [p(X_1 = s_1, T_1 = t)(1-\alpha)]^{1-z}
\end{aligned}
$$

Now treating $p(s_1, t, z; \zeta)$ as function of random variables $S_1, T$ and $Z$ and taking expectation w.r.t. the distribution of $T$ and $Z$ given $S_1 = s_1$ and $\bar{\zeta}$.

$$
\begin{aligned}
&\mathbb{E}\big[\log p(S_1, T, Z; \zeta) | S_1 = s_1; \bar{\zeta}\big] \\
&\quad = \mathbb{E}\big[Z(\log\alpha + \log p(X_c = s_1, T_c = t; \theta_c)) | S_1 = s_1; \bar{\zeta}\big] + \mathbb{E}\big[(1 - Z)(\log(1-\alpha) + \log p(X_1 = s_1, T_1 = t; \theta_1)) | S_1 = s_1; \bar{\zeta}\big] \\
&\quad \stackrel{\zeta}{=} \bar{p}_c(s_1)\bigg(\log\alpha - \frac{1}{2} q\big(s_1, v(s_1, \bar{\theta}_c), w(s_1, \bar{\theta}_c), \theta_c\big)\bigg) + \bar{p}_1(s_1)\bigg(\log(1-\alpha) - \frac{1}{2} q\big(s_1, v(s_1, \bar{\theta}_1), w(s_1, \bar{\theta}_1), \theta_1\big)\bigg),
\end{aligned}
$$

where the last line is obtained by first applying Lemma 3 and then Lemma 2.

**Lemma** 5. *Let $S_2$ be the random variable corresponding to the second score distributed as* $S_2 \stackrel{d}{=} Y_1 X_1 + Y_2 X_2 + Y_c X_c$, *where* $X_c \sim \text{SN}(\theta_c), X_1 \sim \text{SN}(\theta_1), X_2 \sim \text{SN}(\theta_2)$, $Y = [Y_1, Y_2, Y_c] \sim \text{Categorical}([\alpha, 1-\alpha-\beta, \beta])$, $\alpha, \beta \in [0,1]$ *and* $\alpha + \beta < 1$. *Let* $T_c, T_1, T_2 \sim \text{HN}(0,1)$ *and* $U_c, U_1, U_2 \sim \text{N}(0,1)$ *be related to* $X_c, X_1$ *and* $X_2$ *respectively by the probabilistic representation of* SN *random variable as* $X_c \stackrel{d}{=} \mu_c + \Delta_c T_c + \Gamma_c^{1/2} U_c$, $X_1 \stackrel{d}{=} \mu_1 + \Delta_1 T_1 + \Gamma_1^{1/2} U_1$ *and* $X_2 \stackrel{d}{=} \mu_2 + \Delta_2 T_2 + \Gamma_2^{1/2} U_2$. *Further, let* $T \stackrel{d}{=} Y_1 T_1 + Y_2 T_1 + Y_c T_c$. *Then for the joint density of* $S_2, T, Y$ *given by* $p(s_2, t, y; \zeta)$,

$$
\begin{aligned}
\mathbb{E}\big[\log p(S_2, T, Y; \zeta) | S_2 = s_2; \bar{\zeta}\big] \stackrel{\zeta}{=} \;& \bar{r}_1(s_2)\bigg(\log\alpha - \frac{1}{2} q\big(s_2, v(s_2, \bar{\theta}_1), w(s_2, \bar{\theta}_1), \theta_1\big)\bigg) \\
&+ \bar{r}_2(s_2)\bigg(\log(1-\alpha-\beta) - \frac{1}{2} q\big(s_2, v(s_2, \bar{\theta}_2), w(s_2, \bar{\theta}_2), \theta_2\big)\bigg) \\
&+ \bar{r}_c(s_2)\bigg(\log\beta - \frac{1}{2} q\big(s_2, v(s_2, \bar{\theta}_c), w(s_2, \bar{\theta}_c), \theta_c\big)\bigg),
\end{aligned}
$$

*where $\zeta$ serves as placeholder for $(\alpha, \beta, \theta_c, \theta_1, \theta_2)$; the expectation is taken w.r.t. the distribution of $T, Y$ given $S_2 = s_2$ with $\bar{\zeta}$ used as the parameter for the conditional distribution;*

$$
\begin{aligned}
\bar{r}_1(s_2) &= p\big(Y_1 = 1 | S_2 = s_2, \bar{\zeta}\big) \\
\bar{r}_2(s_2) &= p\big(Y_2 = 1 | S_2 = s_2, \bar{\zeta}\big) \\
\bar{r}_c(s_2) &= p\big(Y_c = 1 | S_2 = s_2, \bar{\zeta}\big).
\end{aligned}
$$

Proof. The joint distribution of $S_2, T, Y$ can be written as

$$\begin{aligned} p(s_2,t,y) &= p(s_2,t,Y_1=1])^{y_1} p(s_2,t,Y_2=1)^{y_2} p(s_2,t,Y_c=1)^{y_c} \\ &= [p(s_2,t|Y_1=1)p(Y_1=1)]^{y_1} [p(s_2,t|Y_2=1)p(Y_2=1)]^{y_2} [p(s_2,t|Y_c=1)p(Y_c=1)]^{y_c} \\ &= [p(X_1=s_2,T_1=t)\alpha]^{y_1} [p(X_2=s_2,T_2=t)(1-\alpha-\beta)]^{y_2} [p(X_c=s_2,T_c=t)\beta]^{y_c} \end{aligned}$$

Now treating $p(s_2,t,y;\zeta)$ as function of random variables $s_2, T$ and $Y$ and taking expectation w.r.t. the distribution of $T, Y$ given $S_2 = s_2$ and $\bar{\zeta}$.

$$\begin{aligned} \mathbb{E}\big[\log p(S_2,T,Y;\zeta)|S_2=s_2;\bar{\zeta}\big] &= \mathbb{E}\big[Y_1(\log\alpha + \log p(X_1=s_2,T_1=t;\theta_1))|S_2=s_2;\bar{\zeta}\big] \\ &+ \mathbb{E}\big[Y_2(\log(1-\alpha-\beta) + \log p(X_2=s_2,T_2=t;\theta_2))|S_2=s_2;\bar{\zeta}\big] \\ &+ \mathbb{E}\big[Y_c(\log\beta + \log p(X_c=s_2,T_c=t;\theta_c))|S_2=s_2;\bar{\zeta}\big] \end{aligned} \tag{3}$$

Now, $S_2$ can be expressed in the form required by Lemma 3 with $Y_i$ $(i=1,2,c)$ replacing $Z$ (in Lemma 3) as follows

$$\begin{aligned} S_2 &\overset{d}{=} Y_1X_1 + (1-Y_1)(Y_2X_2 + Y_cX_c), \\ S_2 &\overset{d}{=} Y_2X_2 + (1-Y_2)(Y_1X1 + Y_cX_c), \\ S_2 &\overset{d}{=} Y_cX_c + (1-Y_c)(Y_1X1 + Y_2X_2). \end{aligned}$$

First applying Lemma 3 to Equation 3 and then applying Lemma 2 gives

$$\begin{aligned} \mathbb{E}\big[\log p(S_2,T,Y;\zeta)|S_2=s_2;\bar{\zeta}\big] &\overset{\zeta}{=} \bar{r}_1(s_2)\Big(\log\alpha - \frac{1}{2}q\big(s_2, v(s_2,\bar{\theta}_1), w(s_2,\bar{\theta}_1), \theta_1\big)\Big) \\ &+ \bar{r}_2(s_2)\Big(\log(1-\alpha-\beta) - \frac{1}{2}q\big(s_2, v(s_2,\bar{\theta}_2), w(s_2,\bar{\theta}_2), \theta_2\big)\Big) \\ &+ \bar{r}_c(s_2)\Big(\log\beta - \frac{1}{2}q\big(s_2, v(s_2,\bar{\theta}_c), w(s_2,\bar{\theta}_c), \theta_c\big)\Big). \end{aligned}$$

## 2 Derivation of the parameter update equations

### 2.1 Partial derivatives of the $q$-function

$$\begin{aligned} \frac{\partial}{\partial\mu}q(x,t,\tau,\theta) &= \frac{2\mu - 2(x-\Delta t)}{\Gamma} \\ \frac{\partial}{\partial\Delta}q(x,t,\tau,\theta) &= \frac{2\Delta\tau - 2(x-\mu)t}{\Gamma} \\ \frac{\partial}{\partial\Gamma}q(x,t,\tau,\theta) &= \frac{1}{\Gamma} - \frac{(x-\mu)^2 - 2\Delta(x-\mu)t + \Delta^2\tau}{\Gamma^2} \end{aligned}$$

### 2.2 1SMix

The pdf of $S_1$ (top score) under the 1SMix model is given by

$$f_1(x) = \alpha f_{\text{SN}}(x;\theta_c) + (1-\alpha) f_{\text{SN}}(x,\theta_1).$$

The log-likelihood of $\mathbb{S}_1$ (containing all top scores) is given by

$$\mathcal{L}(\mathbb{S}_1;\zeta) = \frac{1}{|\mathbb{S}_1|}\sum_{s_1\in\mathbb{S}_1} \log f_1(s_1).$$

We obtain maximum likelihood estimate of $\zeta$ by indirectly maximizing the log-likelihood using the Expectation Maximization (EM) approach.
To derive the EM algorithm, notice that the 1SMix model for $S_1$ can be alternatively expressed as that in Lemma 4. Let ${\mathbb{S}_1}^{\mathfrak{C}}$ be a partially observed sample containing triples of the form $(s_1, t, z)$ for all $s_1 \in \mathbb{S}_1$, where $t$ and $z$ are the unobserved values for $T$ and $Z$ corresponding to $S_1$. We will use

${\mathbb{S}_1}^{\mathfrak{C}}$ as the complete data in the Expectation Maximization (EM) framework. The so called "Q-function" can be derived as

$$
\begin{aligned}
Q(\zeta|\bar{\zeta}) &= \mathbb{E}\Big[\log p\Big({\mathbb{S}_1}^{\mathfrak{C}};\zeta)\Big)\Big|\mathbb{S}_1,\bar{\zeta}\Big] \\
&= \mathbb{E}\Bigg[\log \prod_{(s_1,t,z)\in{\mathbb{S}_1}^{\mathfrak{C}}} p(s_1,t,z;\zeta)\Bigg|\mathbb{S}_1,\bar{\zeta}\Bigg] \\
&= \mathbb{E}\Bigg[\sum_{(s_1,t,z)\in{\mathbb{S}_1}^{\mathfrak{C}}} \log p(s_1,t,z;\zeta)\Bigg|\mathbb{S}_1,\bar{\zeta}\Bigg] \\
&= \sum_{s_1\in\mathbb{S}_1} \mathbb{E}\big[\log p(s_1,t,z;\zeta)|S_1=s_1,\bar{\zeta}\big] \\
&\overset{\zeta}{=} \sum_{s_1\in\mathbb{S}_1} \bar{p}_c(s_1)\Big(\log\alpha - \frac{1}{2}q\big(s_1,v(s_1,\bar{\theta}_c),w(s_1,\bar{\theta}_c),\theta_c\big)\Big) + \sum_{s_1\in\mathbb{S}_1} \bar{p}_1(s_1)\Big(\log(1-\alpha) - \frac{1}{2}q\big(s_1,v(s_1,\bar{\theta}_1),w(s_1,\bar{\theta}_1),\theta_1\big)\Big)
\end{aligned}
$$

The update equations are obtained by taking the partial derivatives of $Q(\zeta|\bar{\zeta})$ w.r.t. $\alpha,\mu_c,\mu_1,\Delta_c,\Delta_1,\Gamma_c$ and $\Gamma_1$ and equating them to 0.

### 2.3 2SMix

The pdfs of $S_1$ (top score) and $S_2$ (second score) under the 2SMix model are given by

$$
\begin{aligned}
f_1(x) &= \alpha f_{\mathrm{SN}}(x;\theta_c) + (1-\alpha) f_{\mathrm{SN}}(x,\theta_1), \\
f_2(x) &= \alpha f_{\mathrm{SN}}(x;\theta_1) + (1-\alpha-\beta) f_{\mathrm{SN}}(x,\theta_2) + \beta f_{\mathrm{SN}}(x,\theta_c),
\end{aligned}
$$

respectively. The combined log-likelihood of $\mathbb{S}_1$ (containing all top scores) and $\mathbb{S}_2$ (containing all second scores) is given by

$$
\mathcal{L}(\mathbb{S}_1,\mathbb{S}_2;\zeta) = \frac{1}{|\mathbb{S}_1|}\sum_{s_1\in\mathbb{S}_1}\log f_1(s_1) + \frac{1}{|\mathbb{S}_2|}\sum_{s_2\in\mathbb{S}_2}\log f_2(s_2).
$$

We obtain maximum likelihood estimate of $\zeta$ by indirectly maximizing the log-likelihood using the Expectation Maximization (EM) approach.
To derive the EM algorithm, notice that the 2SMix model for $S_1$ and $S_2$ can be alternatively expressed as that in Lemma 4 and Lemma 5, respectively. The parameters $\alpha,\theta_c,\theta_1$ are shared between the models for $S_1$ and $S_2$. Let ${\mathbb{S}_1}^{\mathfrak{C}}$ be a partially observed sample containing triples of the form $(s_1,t,z)$ for all $s_1\in\mathbb{S}_1$, where $t$ and $z$ are the unobserved values for $T$ and $Z$ corresponding to $S_1$ according to Lemma 4. Let ${\mathbb{S}_2}^{\mathfrak{C}}$ be a partially observed sample containing triples of the form $(s_2,t,y)$ for all $s_2\in\mathbb{S}_2$, where $t$ and $y$ are the unobserved values for $T$ and $Y$ corresponding to $S_2$ according to Lemma 5. We will use ${\mathbb{S}_1}^{\mathfrak{C}}$ and ${\mathbb{S}_2}^{\mathfrak{C}}$ as the complete data in the Expectation Maximization (EM) framework. The so called "Q-function" can be derived as

$$
\begin{aligned}
Q(\zeta|\bar{\zeta}) &= \mathbb{E}\Big[\log p\Big({\mathbb{S}_1}^{\mathfrak{C}},{\mathbb{S}_2}^{\mathfrak{C}};\zeta)\Big)\Big|\mathbb{S}_1,\mathbb{S}_2\bar{\zeta}\Big] \\
&= \mathbb{E}\Big[\log p\Big({\mathbb{S}_1}^{\mathfrak{C}};\zeta\Big)\Big|\mathbb{S}_1\bar{\zeta}\Big] + \mathbb{E}\Big[\log p\Big({\mathbb{S}_2}^{\mathfrak{C}};\zeta\Big)\Big|\mathbb{S}_2\bar{\zeta}\Big] \\
&= \mathbb{E}\Bigg[\log \prod_{(s_1,t,z)\in{\mathbb{S}_1}^{\mathfrak{C}}} p(s_1,t,z;\zeta)\Bigg|\mathbb{S}_1,\bar{\zeta}\Bigg] + \mathbb{E}\Bigg[\log \prod_{(s_2,t,y)\in{\mathbb{S}_2}^{\mathfrak{C}}} p(s_2,t,y;\zeta)\Bigg|\mathbb{S}_2,\bar{\zeta}\Bigg] \\
&= \mathbb{E}\Bigg[\sum_{(s_1,t,z)\in{\mathbb{S}_1}^{\mathfrak{C}}} \log p(s_1,t,z;\zeta)\Bigg|\mathbb{S}_1,\bar{\zeta}\Bigg] + \mathbb{E}\Bigg[\sum_{(s_2,t,y)\in{\mathbb{S}_2}^{\mathfrak{C}}} \log p(s_2,t,y;\zeta)\Bigg|\mathbb{S}_2,\bar{\zeta}\Bigg] \\
&= \sum_{s_1\in\mathbb{S}_1} \mathbb{E}\big[\log p(s_1,t,z;\zeta)|S_1=s_1,\bar{\zeta}\big] + \sum_{s_2\in\mathbb{S}_2} \mathbb{E}\big[\log p(s_2,t,y;\zeta)|S_2=s_2,\bar{\zeta}\big] \\
&\overset{\zeta}{=} \sum_{s_1\in\mathbb{S}_1} \bar{p}_c(s_1)\Big(\log\alpha - \frac{1}{2}q\big(s_1,v(s_1,\bar{\theta}_c),w(s_1,\bar{\theta}_c),\theta_c\big)\Big) + \sum_{s_1\in\mathbb{S}_1} \bar{p}_1(s_1)\Big(\log(1-\alpha) - \frac{1}{2}q\big(s_1,v(s_1,\bar{\theta}_1),w(s_1,\bar{\theta}_1),\theta_1\big)\Big) \\
&\quad + \sum_{s_2\in\mathbb{S}_2} \bar{r}_1(s_2)\Big(\log\alpha - \frac{1}{2}q\big(s_2,v(s_2,\bar{\theta}_1),w(s_2,\bar{\theta}_1),\theta_1\big)\Big) + \sum_{s_2\in\mathbb{S}_2} \bar{r}_2(s_2)\Big(\log(1-\alpha-\beta) - \frac{1}{2}q\big(s_2,v(s_2,\bar{\theta}_2),w(s_2,\bar{\theta}_2),\theta_2\big)\Big) \\
&\quad + \sum_{s_2\in\mathbb{S}_2} \bar{r}_c(s_2)\Big(\log\beta - \frac{1}{2}q\big(s_2,v(s_2,\bar{\theta}_c),w(s_2,\bar{\theta}_c),\theta_c\big)\Big),
\end{aligned}
$$

The update equations are obtained by taking the partial derivatives of $Q(\zeta|\bar{\zeta})$ w.r.t. $\alpha,\beta,\mu_c,\mu_1,\mu_2,\Delta_c,\Delta_1,\Delta_2,\Gamma_c,\Gamma_1$ and $\Gamma_2$ and equating them to 0. To obtain a simpler update equation for $\alpha$, we use the reparametrization: $\beta=(1-\alpha)c_1$ and $1-\alpha-\beta=(1-\alpha)c_2$, where $c_1,c_2\in[0,1]$ and $c_1+c_2=1$. Similarly, to obtain a simpler update equation for $\beta$ we use the reparametrization: $\alpha=(1-\beta)c_3$ and $1-\alpha-\beta=(1-\beta)c_4$, where $c_3,c_4\in[0,1]$ and $c_3+c_4=1$.

## 3 Method of moments estimator for SN parameters

Given a sample $\mathbb{S}$ from SN$(\mu, \omega, \lambda)$, the method of moment estimator is given by the following equations.
**SN Method of Moments** (Arnold *et al.*, 1993):

$$\hat{\delta} = \mathrm{sgn}(m_3)\left(a_1^2 + m_2({}^{b_1}/_{|m_3|})^{2/3}\right)^{-1/2},$$

$$\hat{\omega}^2 = \frac{m_2}{1 - a_1^2\hat{\delta}^2},$$

$$\hat{\mu} = m_1 - a_1\hat{\delta}\hat{\omega},$$

where $a_1 = \sqrt{2/\pi}$, $b_1 = (4/\pi - 1)a_1$, $m_1 = 1/|\mathbb{S}| \sum_{s\in\mathbb{S}} s$, $m_2 = 1/(|\mathbb{S}|-1) \sum_{s\in\mathbb{S}}(s - m_1)^2$ and $m_3 = 1/(|\mathbb{S}|-1) \sum_{s\in\mathbb{S}}(s - m_1)^3$.

## 4 Supporting Results

### 4.1 PRIDE Datasets

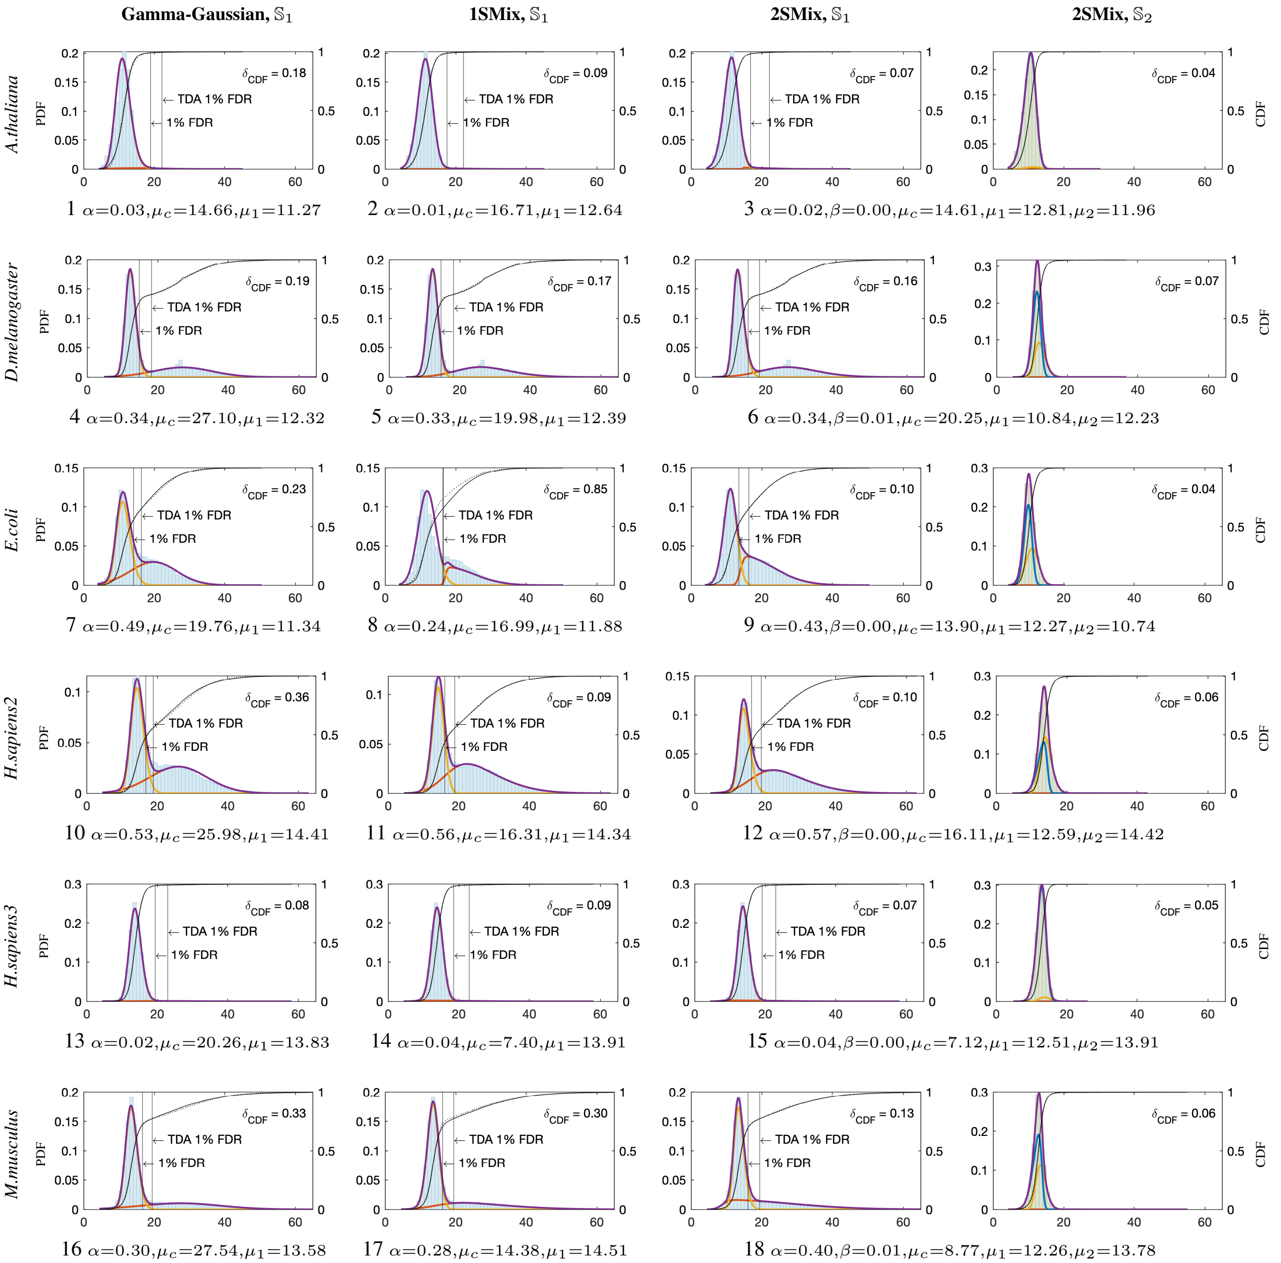


1 $\alpha$=0.03,$\mu_c$=14.66,$\mu_1$=11.27
2 $\alpha$=0.01,$\mu_c$=16.71,$\mu_1$=12.64
3 $\alpha$=0.02,$\beta$=0.00,$\mu_c$=14.61,$\mu_1$=12.81,$\mu_2$=11.96

4 $\alpha$=0.34,$\mu_c$=27.10,$\mu_1$=12.32
5 $\alpha$=0.33,$\mu_c$=19.98,$\mu_1$=12.39
6 $\alpha$=0.34,$\beta$=0.01,$\mu_c$=20.25,$\mu_1$=10.84,$\mu_2$=12.23

7 $\alpha$=0.49,$\mu_c$=19.76,$\mu_1$=11.34
8 $\alpha$=0.24,$\mu_c$=16.99,$\mu_1$=11.88
9 $\alpha$=0.43,$\beta$=0.00,$\mu_c$=13.90,$\mu_1$=12.27,$\mu_2$=10.74

10 $\alpha$=0.53,$\mu_c$=25.98,$\mu_1$=14.41
11 $\alpha$=0.56,$\mu_c$=16.31,$\mu_1$=14.34
12 $\alpha$=0.57,$\beta$=0.00,$\mu_c$=16.11,$\mu_1$=12.59,$\mu_2$=14.42

13 $\alpha$=0.02,$\mu_c$=20.26,$\mu_1$=13.83
14 $\alpha$=0.04,$\mu_c$=7.40,$\mu_1$=13.91
15 $\alpha$=0.04,$\beta$=0.00,$\mu_c$=7.12,$\mu_1$=12.51,$\mu_2$=13.91

16 $\alpha$=0.30,$\mu_c$=27.54,$\mu_1$=13.58
17 $\alpha$=0.28,$\mu_c$=14.38,$\mu_1$=14.51
18 $\alpha$=0.40,$\beta$=0.01,$\mu_c$=8.77,$\mu_1$=12.26,$\mu_2$=13.78

**Gamma-Gaussian, $\mathbb{S}_1$** **1SMix, $\mathbb{S}_1$** **2SMix, $\mathbb{S}_1$** **2SMix, $\mathbb{S}_2$**

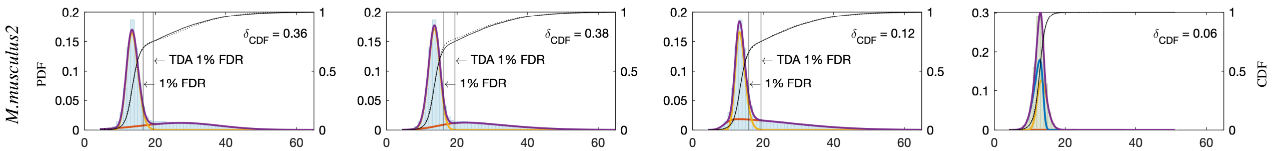


19 $\alpha=0.32,\mu_c=27.15,\mu_1=13.61$ 20 $\alpha=0.30,\mu_c=14.97,\mu_1=14.59$ 21 $\alpha=0.43,\beta=0.01,\mu_c=8.97,\mu_1=12.27,\mu_2=13.78$

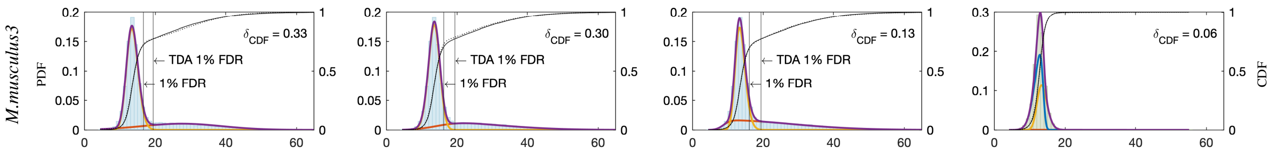


22 $\alpha=0.30,\mu_c=27.54,\mu_1=13.58$ 23 $\alpha=0.28,\mu_c=14.38,\mu_1=14.51$ 24 $\alpha=0.40,\beta=0.01,\mu_c=8.77,\mu_1=12.26,\mu_2=13.78$

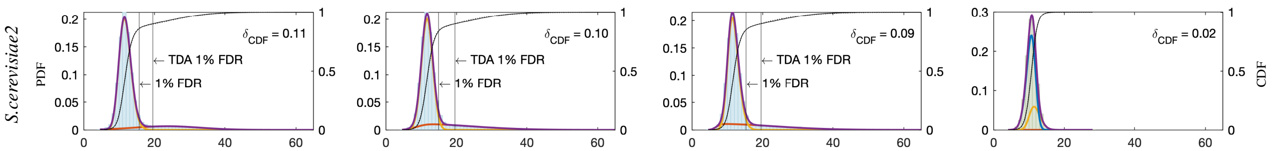


25 $\alpha=0.15,\mu_c=23.66,\mu_1=11.75$ 26 $\alpha=0.21,\mu_c=8.69,\mu_1=11.74$ 27 $\alpha=0.22,\beta=0.00,\mu_c=6.87,\mu_1=10.29,\mu_2=11.69$

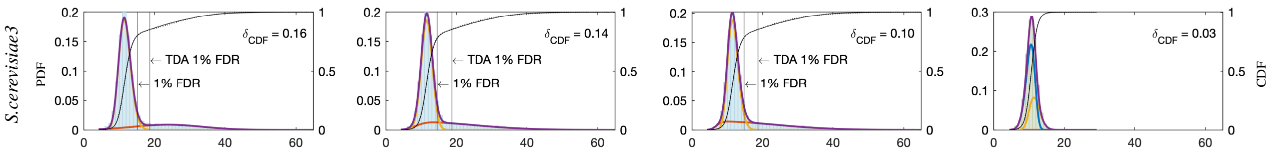


28 $\alpha=0.22,\mu_c=23.87,\mu_1=11.68$ 29 $\alpha=0.27,\mu_c=8.52,\mu_1=11.66$ 30 $\alpha=0.30,\beta=0.00,\mu_c=6.95,\mu_1=10.29,\mu_2=11.61$

## 4.2 NIST Datasets

**Gamma-Gaussian, $\mathbb{S}_1$** **1SMix, $\mathbb{S}_1$** **2SMix, $\mathbb{S}_1$** **2SMix, $\mathbb{S}_2$**

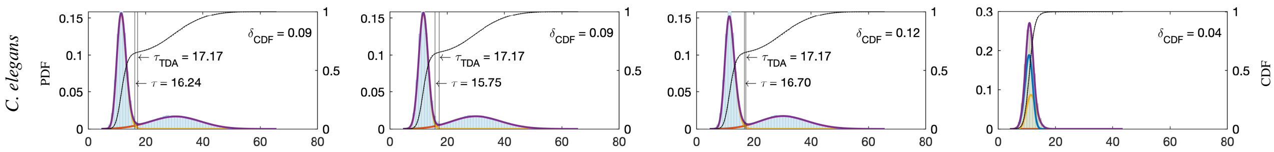


31 $\alpha=0.37,\mu_c=30.47,\mu_1=11.69$ 32 $\alpha=0.37,\mu_c=24.69,\mu_1=11.78$ 33 $\alpha=0.36,\beta=0.00,\mu_c=24.74,\mu_1=10.14,\mu_2=11.73$

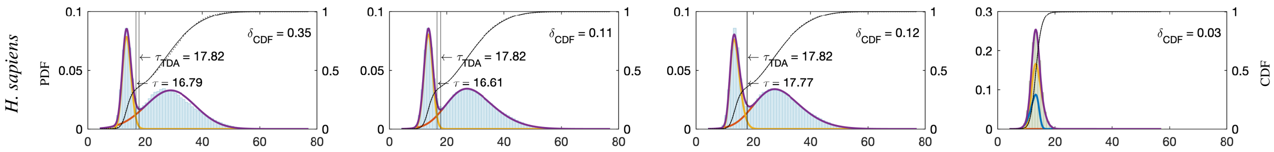


34 $\alpha=0.71,\mu_c=28.85,\mu_1=13.65$ 35 $\alpha=0.70,\mu_c=20.60,\mu_1=13.79$ 36 $\alpha=0.69,\beta=0.00,\mu_c=21.09,\mu_1=11.97,\mu_2=14.39$

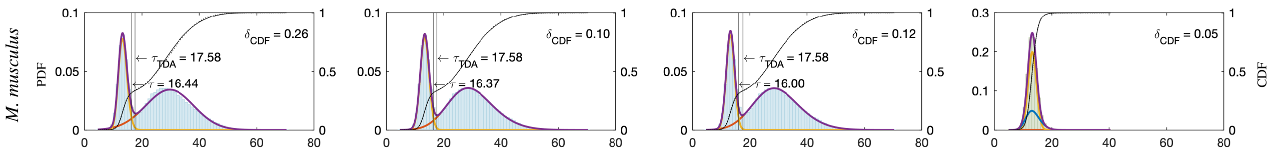


37 $\alpha=0.71,\mu_c=29.64,\mu_1=13.37$ 38 $\alpha=0.70,\mu_c=22.44,\mu_1=13.40$ 39 $\alpha=0.71,\beta=0.00,\mu_c=22.40,\mu_1=13.33,\mu_2=11.23$

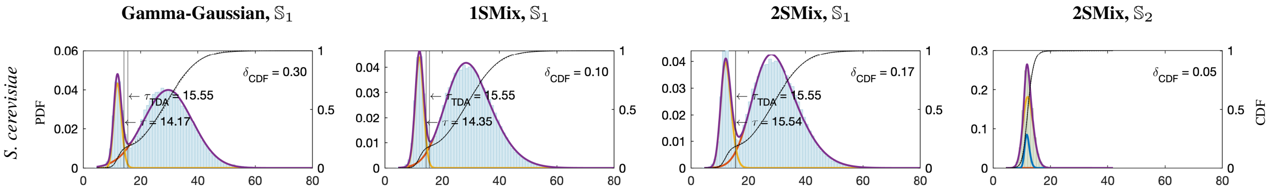


40 $\alpha$=0.86,$\mu_c$=29.56,$\mu_1$=12.03 41 $\alpha$=0.84,$\mu_c$=22.09,$\mu_1$=11.70 42 $\alpha$=0.82,$\beta$=0.00,$\mu_c$=21.86,$\mu_1$=10.75,$\mu_2$=11.10

## 4.3 HeLa Datasets

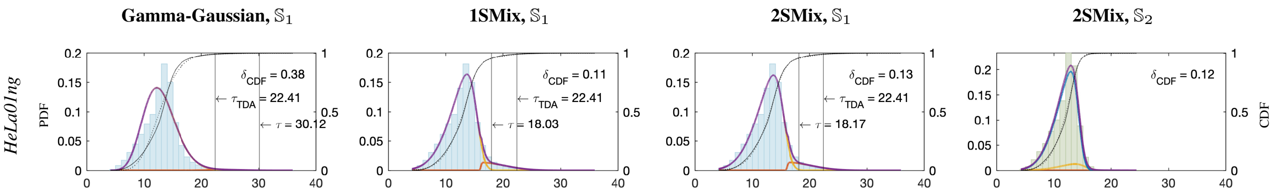


43 $\alpha$=0.01,$\mu_c$=24.45,$\mu_1$=12.84 44 $\alpha$=0.07,$\mu_c$=16.09,$\mu_1$=15.38 45 $\alpha$=0.07,$\beta$=0.00,$\mu_c$=16.05,$\mu_1$=15.39,$\mu_2$=14.28

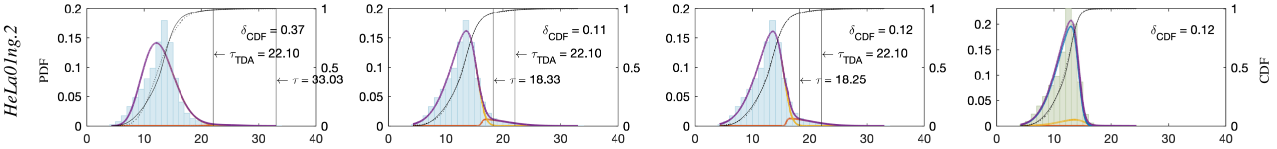


46 $\alpha$=0.01,$\mu_c$=24.48,$\mu_1$=12.75 47 $\alpha$=0.06,$\mu_c$=16.23,$\mu_1$=15.34 48 $\alpha$=0.07,$\beta$=0.00,$\mu_c$=15.87,$\mu_1$=15.32,$\mu_2$=14.26

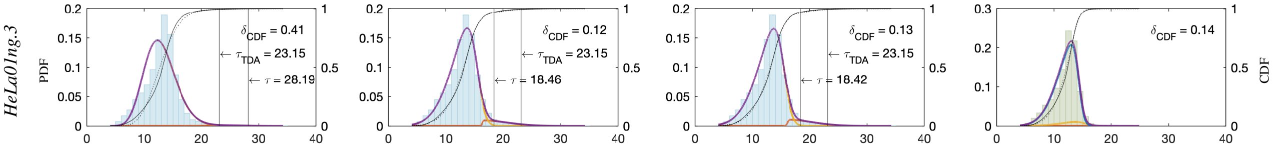


49 $\alpha$=0.01,$\mu_c$=24.94,$\mu_1$=12.89 50 $\alpha$=0.05,$\mu_c$=16.35,$\mu_1$=15.46 51 $\alpha$=0.06,$\beta$=0.00,$\mu_c$=16.09,$\mu_1$=15.46,$\mu_2$=14.28

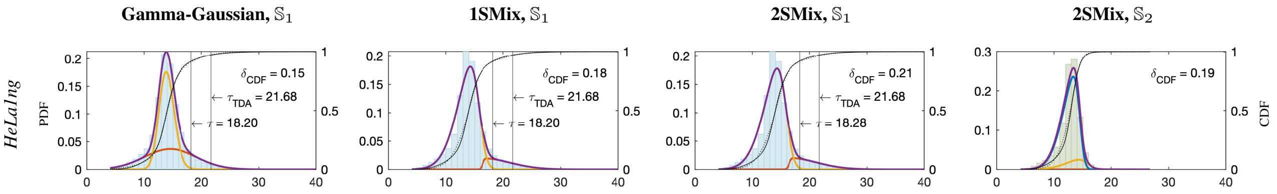


52 $\alpha$=0.42,$\mu_c$=14.56,$\mu_1$=13.95 53 $\alpha$=0.12,$\mu_c$=16.45,$\mu_1$=15.78 54 $\alpha$=0.12,$\beta$=0.00,$\mu_c$=16.41,$\mu_1$=15.82,$\mu_2$=14.45

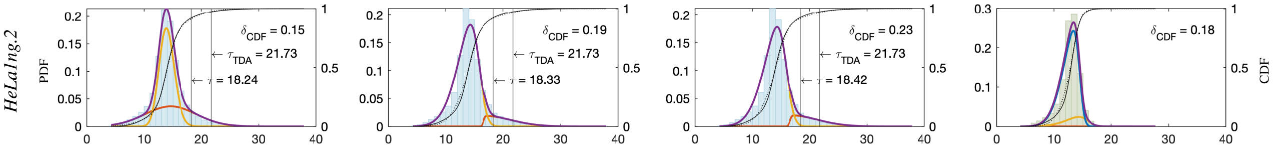


55 $\alpha$=0.41,$\mu_c$=14.64,$\mu_1$=13.97 56 $\alpha$=0.11,$\mu_c$=16.61,$\mu_1$=15.80 57 $\alpha$=0.12,$\beta$=0.00,$\mu_c$=16.57,$\mu_1$=15.84,$\mu_2$=14.43

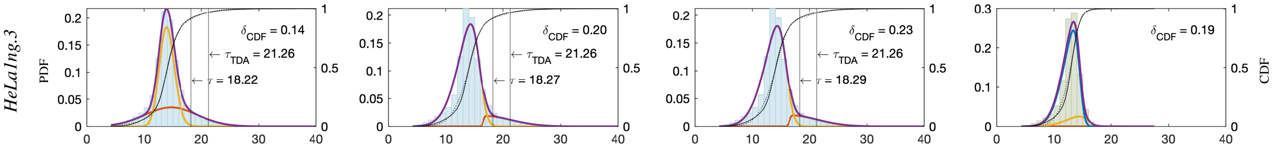


58 $\alpha$=0.40,$\mu_c$=14.71,$\mu_1$=14.00 59 $\alpha$=0.11,$\mu_c$=16.56,$\mu_1$=15.81 60 $\alpha$=0.12,$\beta$=0.00,$\mu_c$=16.49,$\mu_1$=15.85,$\mu_2$=14.43

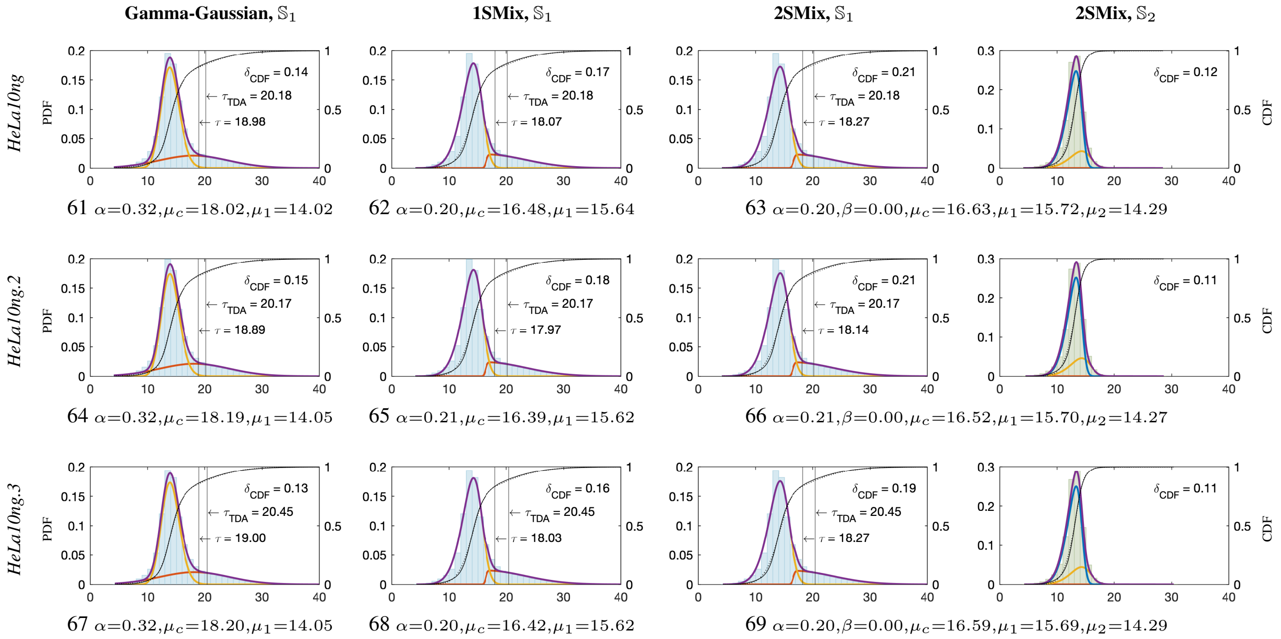


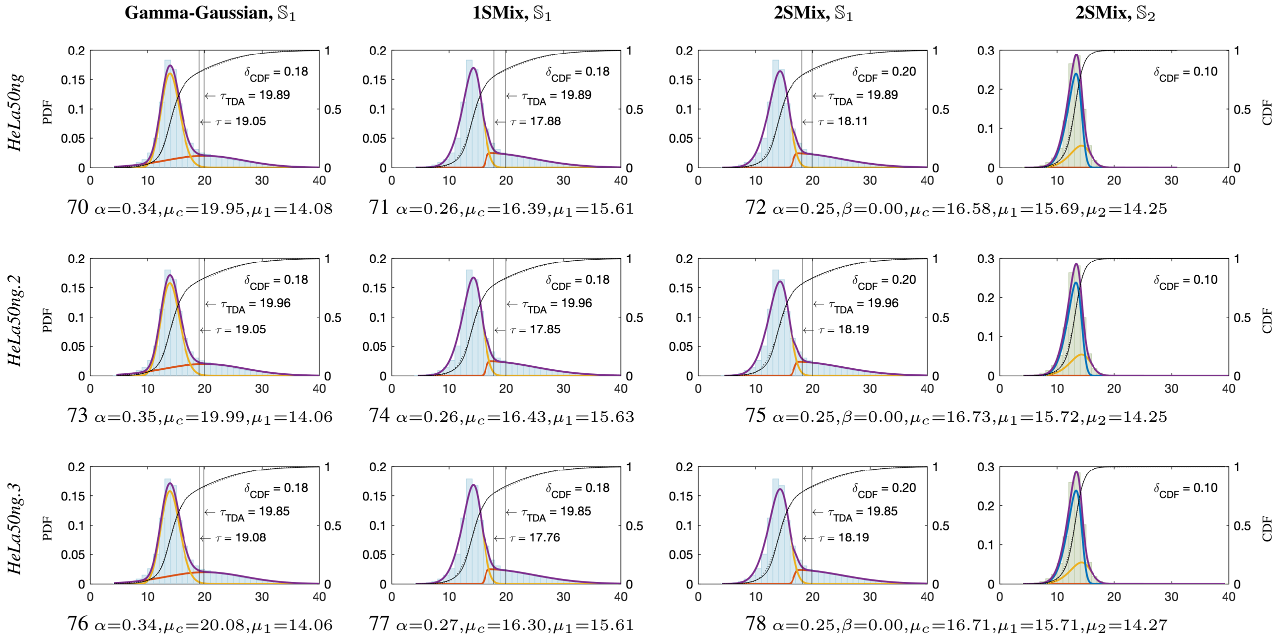


### 4.4 All Results

## References

Arnold, B. C. *et al.* (1993). The nontruncated marginal of a truncated bivariate normal distribution. *Psychometrika*, **58**(3), 471–488.

Johnson, N. L. and Kotz, S. (1970). *Distributions in Statistics: Continuous Univariate Distributions: Vol.: 1*. Houghton Mifflin.

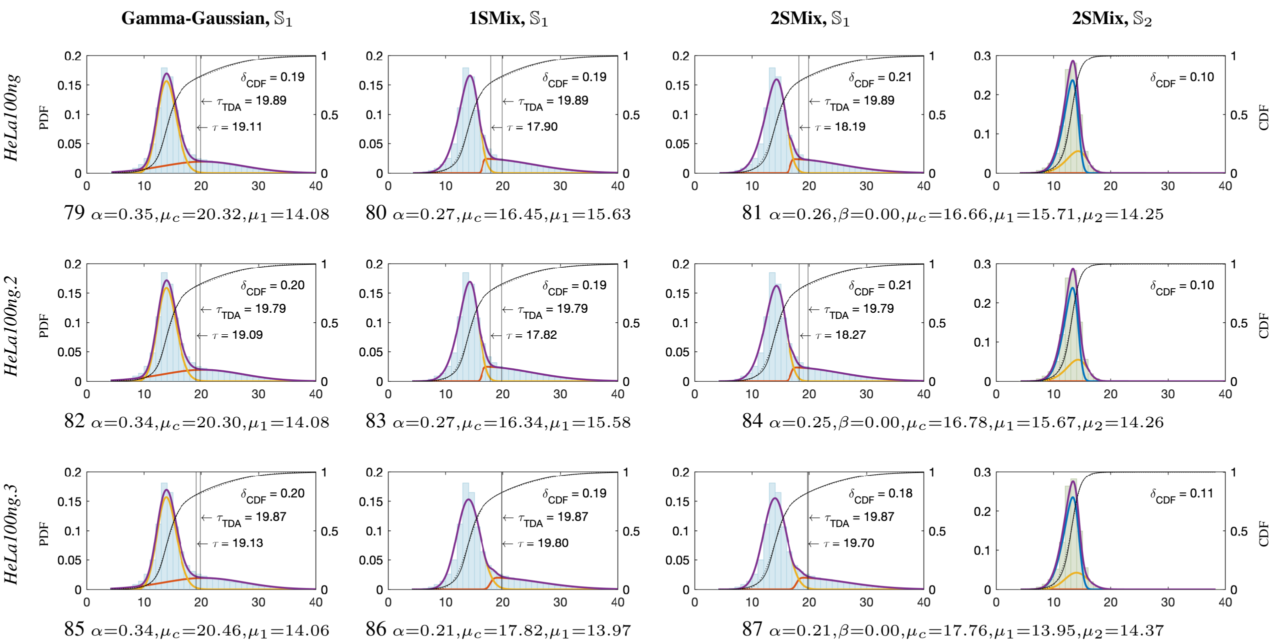


Table 1. Results for all experiments. # hits is the number of identified peptides above 1% FDR threshold; $\tau$ is the 1% FDR threshold; $\delta_{\text{CDF}}$ is the distance between empirical and estimated cdf; $\ell\ell_1$ is the log-likelihood on $\mathbb{S}_1$; $\ell\ell_{1,2}$ is the log-likelihood on $\mathbb{S}_1$ and $\mathbb{S}_2$ together.

| Dataset | | TDA | | Gamma-Gaussian DFA | | | | 1SMix DFA | | | | 2SMix DFA | | | | |
|---|---|---|---|---|---|---|---|---|---|---|---|---|---|---|---|---|
| | | # hits | $\tau$ | # hits | $\tau$ | $\delta_{\text{CDF}}$ | $\ell\ell_1$ | # hits | $\tau$ | $\delta_{\text{CDF}}$ | $\ell\ell_1$ | # hits | $\tau$ | $\delta_{\text{CDF}}$ | $\ell\ell_1$ | $\ell\ell_{1,2}$ |
| PRIDE | *A. thaliana* | 354 | 22.13 | 433 | 21.17 | 0.182 | -2.2452 | 723 | 18.79 | 0.089 | -2.2256 | 857 | 18.07 | 0.066 | -2.2239 | -4.1987 |
| | *D. melanogaster* | 21425 | 18.23 | 22591 | 16.42 | 0.193 | -2.9175 | 22958 | 16.09 | 0.171 | -2.9172 | 22181 | 16.90 | 0.162 | -2.9146 | -4.7033 |
| | *E. coli* | 15001 | 16.33 | 14407 | 16.72 | 0.226 | -3.0582 | 11070 | 18.95 | 0.850 | -3.0806 | 16713 | 15.31 | 0.100 | -3.0479 | -4.9211 |
| | *H. sapiens* 1 | 21486 | 18.80 | 21109 | 19.05 | 0.358 | -3.2573 | 22918 | 17.89 | 0.085 | -3.2461 | 22094 | 18.41 | 0.099 | -3.2461 | -5.1892 |
| | *H. sapiens* 2 | 247 | 22.89 | 313 | 20.77 | 0.081 | -2.0241 | 401 | 19.68 | 0.087 | -2.0220 | 328 | 20.49 | 0.071 | -2.0188 | -3.7564 |
| | *M. musculus* 1 | 12578 | 19.36 | 13283 | 18.45 | 0.335 | -2.9247 | 13964 | 17.67 | 0.298 | -2.9112 | 13757 | 17.88 | 0.131 | -2.9072 | -4.7852 |
| | *M. musculus* 2 | 16419 | 19.40 | 17431 | 18.40 | 0.361 | -2.9822 | 18192 | 17.70 | 0.375 | -2.9689 | 18115 | 17.76 | 0.124 | -2.9636 | -4.8401 |
| | *M. musculus* 3 | 12578 | 19.36 | 13283 | 18.45 | 0.335 | -2.9247 | 13964 | 17.67 | 0.298 | -2.9112 | 13757 | 17.88 | 0.131 | -2.9072 | -4.7852 |
| | *S. cerevisiae* 1 | 3867 | 19.50 | 4502 | 17.47 | 0.112 | -2.5084 | 5016 | 16.29 | 0.103 | -2.5034 | 4648 | 17.08 | 0.086 | -2.5006 | -4.3121 |
| | *S. cerevisiae* 2 | 5402 | 18.65 | 6010 | 17.11 | 0.158 | -2.6846 | 6653 | 15.94 | 0.140 | -2.6756 | 6271 | 16.53 | 0.104 | -2.6736 | -4.5201 |
| NIST | *C. elegans* | 23224 | 17.17 | 23764 | 16.24 | 0.085 | -3.1058 | 24155 | 15.75 | 0.091 | -3.1070 | 23467 | 16.70 | 0.122 | -3.1061 | -5.0126 |
| | *H. sapiens* | 218487 | 17.82 | 225599 | 16.79 | 0.353 | -3.5219 | 227023 | 16.61 | 0.106 | -3.5154 | 218963 | 17.77 | 0.125 | -3.5167 | -5.4989 |
| | *M. musculus* | 99358 | 17.58 | 102065 | 16.44 | 0.263 | -3.5261 | 102241 | 16.37 | 0.096 | -3.5221 | 103481 | 16.00 | 0.116 | -3.5234 | -5.5007 |
| | *S. cerevisiae* | 75529 | 15.55 | 77385 | 14.17 | 0.301 | -3.6286 | 77067 | 14.35 | 0.100 | -3.6214 | 75606 | 15.54 | 0.172 | -3.6244 | -5.5864 |
| HeLa Cell Digest | HeLa01ng | 218 | 22.41 | 9 | 30.12 | 0.378 | -2.5319 | 1058 | 18.03 | 0.115 | -2.4826 | 997 | 18.17 | 0.126 | -2.4827 | -4.6226 |
| | HeLa01ng.2 | 255 | 22.10 | 1 | 33.03 | 0.370 | -2.5310 | 895 | 18.33 | 0.110 | -2.4848 | 920 | 18.25 | 0.120 | -2.4849 | -4.6320 |
| | HeLa01ng.3 | 152 | 23.15 | 18 | 28.19 | 0.412 | -2.5027 | 757 | 18.46 | 0.124 | -2.4416 | 771 | 18.42 | 0.135 | -2.4418 | -4.5397 |
| | HeLa1ng | 1314 | 21.68 | 3798 | 18.20 | 0.152 | -2.4335 | 3802 | 18.20 | 0.185 | -2.4433 | 3702 | 18.28 | 0.211 | -2.4436 | -4.3975 |
| | HeLa1ng.2 | 1305 | 21.73 | 3837 | 18.24 | 0.147 | -2.4249 | 3713 | 18.33 | 0.193 | -2.4356 | 3612 | 18.42 | 0.226 | -2.4360 | -4.3732 |
| | HeLa1ng.3 | 1500 | 21.26 | 3812 | 18.22 | 0.140 | -2.4173 | 3748 | 18.27 | 0.203 | -2.4315 | 3733 | 18.29 | 0.228 | -2.4318 | -4.3607 |
| | HeLa10ng | 7480 | 20.18 | 9375 | 18.98 | 0.142 | -2.5938 | 11229 | 18.07 | 0.172 | -2.5961 | 10759 | 18.27 | 0.211 | -2.5967 | -4.4853 |
| | HeLa10ng.2 | 7560 | 20.17 | 9602 | 18.89 | 0.147 | -2.5898 | 11538 | 17.97 | 0.176 | -2.5924 | 11140 | 18.14 | 0.212 | -2.5929 | -4.4620 |
| | HeLa10ng.3 | 7153 | 20.45 | 9299 | 19.00 | 0.133 | -2.5828 | 11284 | 18.03 | 0.165 | -2.5847 | 10760 | 18.27 | 0.194 | -2.5851 | -4.4594 |
| | HeLa50ng | 12312 | 19.89 | 13925 | 19.05 | 0.175 | -2.7327 | 16591 | 17.88 | 0.178 | -2.7305 | 16018 | 18.11 | 0.202 | -2.7311 | -4.6222 |
| | HeLa50ng.2 | 12581 | 19.96 | 14307 | 19.05 | 0.175 | -2.7538 | 17071 | 17.85 | 0.176 | -2.7514 | 16223 | 18.19 | 0.201 | -2.7521 | -4.6550 |
| | HeLa50ng.3 | 12721 | 19.85 | 14165 | 19.08 | 0.179 | -2.7509 | 17208 | 17.76 | 0.176 | -2.7474 | 16160 | 18.19 | 0.197 | -2.7483 | -4.6488 |
| | HeLa100ng | 14009 | 19.89 | 15516 | 19.11 | 0.191 | -2.7702 | 18477 | 17.90 | 0.191 | -2.7670 | 17718 | 18.19 | 0.214 | -2.7678 | -4.6735 |
| | HeLa100ng.2 | 13833 | 19.79 | 15230 | 19.09 | 0.196 | -2.7519 | 18495 | 17.82 | 0.189 | -2.7484 | 17195 | 18.27 | 0.208 | -2.7492 | -4.6437 |
| | HeLa100ng.3 | 13941 | 19.87 | 15449 | 19.13 | 0.198 | -2.7637 | 14090 | 19.80 | 0.188 | -2.7677 | 14279 | 19.70 | 0.177 | -2.7678 | -4.6690 |
